# Supplementary material for: Neural Jump Ordinary Differential Equations: Consistent Continuous-Time Prediction and Filtering
Source: arXiv:2006.04727 source file (2021-04-16)
Supplement: Supplementary file 1 [file NJODE_appendix.tex]

\documentclass{article}

%%%%%%%%%%%%%%%%%%%%%%%%%%%%%%%%%%%%%%%%%%%%%%%%%%%%%%%%%%%%%%%%%%%%%
%% %TODO :
%%%%%%%%%%%%%%%%%%%%%%%%%%%%%%%%%%%%%%%%%%%%%%%%%%%%%%%%%%%%%%%%%%%%%
% 	- combine with ergodic theorem (discuss with robert) 

%%%%%%%%%%%%%%%%%%%%%%%%%%%%%%%%%%%%%%%%%%%%%%%%%%%%%%%%%%%%%%%%%%%%%%
%%% Controlling behavior of output file
%%%%%%%%%%%%%%%%%%%%%%%%%%%%%%%%%%%%%%%%%%%%%%%%%%%%%%%%%%%%%%%%%%%%%%
%%% View Changes in Color or final version (0: Final, 1: Changes)
\def\viewchanges{0}
%%% View Authors (0: No, 1: Yes)
\def\viewauthors{0}
%%% View Keywords (0: No, 1: Yes)

%%% use hyperlinks (0: No, 1: Yes)
\def\usehyperliks{1}
%%% add acknowledgement (0: No, 1: Yes)

%%% view broader impact (0: No, 1: Yes)

%%% preprint (0: No, 1: Yes)
\def\preprint{0}

%%%%%%%%%%%%%%%%%%%%%%%%%%%%%%%%%%%%%%%%%%%%%%%%%%%%%%%%%%%%%%%%%%%%%%
%%%%%%%%%%%%%%%%%%%%%%%%%%%%%%%%%%%%%%%%%%%%%%%%%%%%%%%%%%%%%%%%%%%%%%

% if you need to pass options to natbib, use, e.g.:
%     \PassOptionsToPackage{numbers, compress}{natbib}
% before loading neurips_2020

\if\preprint0
	% ready for submission
	\usepackage{neurips_2020}
\else
	% to compile a preprint version, e.g., for submission to arXiv, add add the
	% [preprint] option:
     \usepackage[preprint]{neurips_2020}
\fi

% to compile a camera-ready version, add the [final] option, e.g.:
%     \usepackage[final]{neurips_2020}

% to avoid loading the natbib package, add option nonatbib:
 %    \usepackage[nonatbib]{neurips_2020}
 
\usepackage{natbib}

\usepackage[utf8]{inputenc} % allow utf-8 input
\usepackage[T1]{fontenc}    % use 8-bit T1 fonts
\usepackage{url}            % simple URL typesetting
\usepackage{booktabs}       % professional-quality tables
\usepackage{amsfonts}       % blackboard math symbols
\usepackage{nicefrac}       % compact symbols for 1/2, etc.
\usepackage{microtype}      % microtypography
\usepackage{amsthm}
\usepackage{amsmath}
\usepackage{bbm}
\usepackage[dvipsnames]{xcolor}

\if\usehyperliks1
	\usepackage[colorlinks, citecolor=blue, linkcolor=magenta]{hyperref}       % hyperlinks
\fi

% Add for algo
\usepackage{graphicx,wrapfig,lipsum}
\usepackage{subfigure}
\usepackage{verbatim}
\usepackage{bm}
\usepackage{adjustbox}
\usepackage{footnote}
\usepackage{algorithm}
\usepackage{algorithmic}

%for references
\usepackage{xr}
\externaldocument{NJODE}

% new commands:

%

 % expectation

%%% chasing changes with colors:
\usepackage[dvipsnames]{xcolor}

\let\del\undefined
\let\com\undefined

%%% display changes in color:
\if\viewchanges1
	
	\newcommand{\del}{\textcolor{red}}
	\newcommand{\com}{\textcolor{orange}}
	
%%% apply changes:
\else
	
	\newcommand{\del}[1]{}
	\newcommand{\com}[1]{}
	
\fi

\title{Theoretical Guarantees for Learning Conditional Expectation using Controlled ODE-RNN\\
- Supplementary Material -}
%Conditional Expectation using ODE-RNN
%Stochastic process Prediction using Controlled ODE-RNN
%conditional expectation using Controlled ODE-RNN
%On-line Prediction using Controlled ODE-RNN

%\title{Approximation Capabilities of controlled ODE-RNN for SDE Processes}

% The \author macro works with any number of authors. There are two commands
% used to separate the names and addresses of multiple authors: \And and \AND.
%
% Using \And between authors leaves it to LaTeX to determine where to break the
% lines. Using \AND forces a line break at that point. So, if LaTeX puts 3 of 4
% authors names on the first line, and the last on the second line, try using
% \AND instead of \And before the third author name.

\begin{document}

\if\viewauthors1
	\author{%
	  Calypso Herrera \quad Florian Krach \quad Josef Teichmann \\
	  Department of Mathematics, 
	  ETH Zurich, Switzerland
	}
%%	\author{%
%	  Calypso Herrera\\
%	  Department of Mathematics\\
%	  ETH Zurich, Switzerland \\
%	  \texttt{calypso.herrera@math.ethz.ch} \\
%	   \And
%	  Florian Krach\\
%	  Department of Mathematics\\
%	  ETH Zurich, Switzerland \\
%	  \texttt{florian.krach@math.ethz.ch} \\
%	   \And
%	  Josef Teichmann\\
%	  Department of Mathematics\\
%	  ETH Zurich, Switzerland \\
%	  \texttt{josef.teichmann@math.ethz.ch} 
%	}
	\maketitle
\else
	\maketitle
	\vspace*{-1.5cm}
\fi

%%% ==================================================================
	\appendix
	\input{NJODE_appendix_raw}

%%% ==================================================================

%%% ==================================================================
\bibliographystyle{unsrtnat}
\bibliography{references}

\end{document}
